# Supplementary material for: BioMistral-NLU: Towards More Generalizable Medical Language Understanding through Instruction Tuning
Source: arXiv:2410.18955 source file (2025-03-09)
Supplement: Supplementary file 1 [file appendix.tex]

\section*{Appendices}

% Please add the following required packages to your document preamble:
% \usepackage{multirow}
\begin{table}[h]
\small
\resizebox{\textwidth}{!}{%
\begin{tabular}{llrl}
\hline
\textbf{Task} & \textbf{dataset} & \textbf{\# instances} & \textbf{Labels} \\ \hline
\multirow{16}{*}{NER} & i2b2 2006DeID & 5,608 & Location, ID, Date, Hospital, Doctor, Contact, Name, Age \\ \cline{2-4}
 & i2b2 2011 & 25,689 & Person, Treatment, Test, Problem \\ \cline{2-4}
 & i2b2 2012 & 7,446 & \begin{tabular}[c]{@{}l@{}}Test, Problem, Frequency, Time, Date, Occurrence, Treatment,\\ Duration, Clinical department\end{tabular} \\ \cline{2-4}
 & i2b2 2014 & 52,462 & ID, Contact, Age, Name, Location, Profession, Date \\ \cline{2-4}
 & GENIA & 15,023 & RNA, DNA, Cell type, Protein, Cell line \\ \cline{2-4}
 & linnaeus & 11,935 & Species \\ \cline{2-4}
 & tmVar & 5,351 & \begin{tabular}[c]{@{}l@{}}Cell Line, SNP, Gene, Protein Mutation, Protein Allele, Species\\ DNA Allele, DNA Mutation, Other Mutation, Acid Change,\end{tabular} \\ \cline{2-4}
 & DrugProt & 17,274 & \begin{tabular}[c]{@{}l@{}}Organism Taxon, Disease Or Phenotypic Feature, Cell Line, \\ Gene Or Gene Product, Sequence Variant, Chemical\end{tabular} \\ \cline{2-4}
 & BioRed & 13,706 & Chemical, Gene \\ \cline{2-4}
 & GNorm & 4,006 & Family Name, Domain Motif, Gene \\ \cline{2-4}
 & NLM-Gene & 5,048 & \begin{tabular}[c]{@{}l@{}}Gene, Gene reference into function (function of a gene), Domain,\\ Steroidogenic acute regulatory protein (a protein coding gene)\end{tabular} \\ \cline{2-4}
 & ClinicalIE\_Med & 105 & Route, Duration, Reason, Dosage, Frequency, Medication \\ \cline{2-4}
 & ClinicalIE\_Status & 105 & Neither medications, Discontinued medications, Active medications \\ \cline{2-4}
 & BC4CHEMD & 30,682 & Chemical \\ \cline{2-4}
 & PubMed PICO & 1,961 & Species, Comparator, Outcome, Intervention, Strain, Induction \\ \cline{2-4}
 & PICO-Data & 36,224 & Participants, Intervention, Outcome \\ \hline
\multirow{3}{*}{EE} & i2b2 2009 & 117,446 & Medication (Dosage, Route, Frequency, Duration, Reason, Context) \\ \cline{2-4}
 & i2b2 2018 & 155,716 & Drug, ADE (Strength, Frequency, Reason, Form, Route, Dosage) \\ \cline{2-4}
 & n2c2 2022 & 36,359 & \begin{tabular}[c]{@{}l@{}}Alcohol, Drug, Tobacco, Employment, Living \\ (time, duration, history, type, amount, frequency)\end{tabular} \\ \hline
\multirow{6}{*}{DC} & i2b2 2006Smoke & 398 & Current smoker/Past smoker/Non-smoker/Unknown \\ \cline{2-4}
 & i2b2 2008 & 17,242 & 10 obesity commodities (Asthma, Depression, ...) \\ \cline{2-4}
 & n2c2 2018 & 2,626 & Different selection criteria for 13 cohorts (Abdominal, English, ...) \\ \cline{2-4}
 & 2024 SemEval2 & 1,700 & Adverse Events, Eligibility, Results, Intervention \\ \cline{2-4}
 & TrialStop & 3,747 & 17 reasons to stop a study (Study staff moved, Another study, ...) \\ \cline{2-4}
 & MTSamples & 3,206 & 48 medical specialties or domains (Bariatrics, Nephrology, ...) \\ \hline
\multirow{5}{*}{RE} & i2b2 2011 & 25,689 & Refers to \\ \cline{2-4}
 & i2b2 2012 & 7,446 & \begin{tabular}[c]{@{}l@{}}Ends by, Happens during, Happens before and overlap, Begins by,\\ Happens before, Happens simultaneously with, Happens after, \\ Overlaps with,\end{tabular} \\ \cline{2-4}
 & EUADR & 318 & Gene-disease association \\ \cline{2-4}
 & DrugProt & 35,624 & \begin{tabular}[c]{@{}l@{}}Antagonist, Agonist, Indirect upregulator, Part of, Agonist activator,\\ Substrate, Activator, Inhibitor, Direct regulator, Agonist inhibitor, \\ Product of, Substrate product of, Indirect downregulator\end{tabular} \\ \cline{2-4}
 & BioRed & 4,328 & \begin{tabular}[c]{@{}l@{}}Drug interaction, Positive correlation, Cotreatment, Comparison, \\ Bind, Conversion, Association, Negative correlation\end{tabular} \\ \hline
\multirow{3}{*}{NLI} & Multi-NLI & 785,404 & Entailment, Contradiction, Neutral \\ \cline{2-4}
 & SNLI & 1,098,734 & Entailment, Contradiction, Neutral \\ \cline{2-4}
 & BioNLI & 23,704 & Entailment, Contradiction, Neutral \\ \hline
STS & SIS-B & 11,018 & 6 similarity scales \\ \hline
\multirow{3}{*}{NLG} & PubMedSum & 1,407 & Article summarization \\ \cline{2-4}
 & CDSR & 436 & Article simplication \\ \cline{2-4}
 & AciDemo & 204 & Dialogue to note summarization \\ \hline
\end{tabular}
}
\setlength{\belowcaptionskip}{-5pt}
\caption{Task labels and number of instances in the MNLU-Instruct datasets. For EE tasks, labels inside () refer to event arguments. }
\label{tab:instruction-tuing_details}
\end{table}

\subsection*{Unified Prompt Format} \label{sec:datasets}
Utilizing the unified prompt format outlined in Table \ref{tab:prompts}, we developed (1) the MNLU-Instruct dataset based on the collection of datasets detailed in Table \ref{tab:instruction-tuing_details}; and (2) the evaluation dataset from BLUE and BLURB utilizing the labels from Table \ref{tab:ner} and \ref{tab:other_tasks}.
In this section, we provide detailed information on dataset creation and examples of the input-output format for each task type.

\subsubsection*{Named entity recognition (NER)} \label{sec:appdix_ner}
We conduct NER at the sentence level, because most NER datasets comprise pre-split sentences. For NER datasets where the medical text is an entire document, we use the SpaCy tokenizer\footnote{https://spacy.io/api/sentencizer} to split the document into sentences. 

Below is an example of the NER input-output pair. The example is from the n2c2 2022 dataset \cite{lybarger20232022}, a shared task focused on extracting social determinants of health from clinical notes.

\centerline{\textit{ - NER Input - }}

Extract all relevant medical named entities faithfully from the medical text below. Focus on identifying the following entities: Living status, Tobacco, Drug, Employment, Alcohol.

Medical text: Denies any IV drug use or any recreational drug use.

\centerline{\textit{ - NER Output - }}
Living status: None

Tobacco: None

Drug: IV drug use ... recreational drug use

Employment: None

Alcohol: None

\subsubsection*{Event extraction (EE)}
The EE task is composed of event trigger extraction (ETE), event argument extraction (EAE), and event argument classification (EAC). ETE uses the same prompting formats as NER. In EAE and EAC, we additionally include two adjacent sentences to provide more context information. Below are examples of the EAE and EAC input-output pairs from the n2c2 2022 dataset \cite{lybarger20232022}

\centerline{\textit{- EAE Input -}}

According to the medical text, what is the Method attribute of the Drug event `IV drug use' in the medical text below? Extract the attribute faithfully from the medical text.

Medical text: ... Currently admits to five drinks of alcohol per week. Denies any IV drug use or any recreational drug use. Divorced with no children. ...

\centerline{\textit{- EAE Output - }}

Drug - Method: IV

\centerline{\textit{ - EAC Input - }}

According to the medical text, what is the Status time attribute of the Drug event `IV drug use' in the medical text below? Choose from the following options.

Medical text: ... Currently admits to five drinks of alcohol per week. Denies any IV drug use or any recreational drug use. Divorced with no children. ...

Options: (A) none (B) past (C) future (D) current

\centerline{\textit{ - EAC Output - }}

Drug - Status time: (A) none

\subsubsection*{Document classification (DC)}
Our document classification task involves classifying a document or sentence into one or multiple pre-defined categories. 

In the i2b2 2006Smoke \cite{uzuner2008identifying} and i2b2 2008 \cite{uzuner2009recognizing} dataset, where the input document is a lengthy clinical note, we first deploy BioMistral to summarize the document. We use the prompt format, 'Summarize the \{\textit{type}\} from the following clinical note.', where \textit{type} is the corresponding DC type label, such as smoking status or asthma status. 

The MTSamples dataset aims to classify a medical report into one of 48 medical specialties or domains \cite{MTSample}. The large number of possible categories results in lengthy prompts.  Instead, in each instance, we include the correct category along with 12 randomly selected negative categories in our prompts for more efficient training.

Below is an example of the DC input-output pair from the TrialStop dataset \cite{razuvayevskaya2023clinical}. 

\centerline{\textit{- DC Input -}}

According to the medical text below, which options best describe reason to stop the study? Choose from the following options. Multiple options can be true.

Medical text: 13 of 15 patients recruited.Study patients responded with no safety signals. Recruitment's slow, timely end of study necessary to keep development timelines.

Options: (A) Insufficient enrollment (B) Logistics resources (C) Business administrative (D) Insufficient data (E) Endpoint met (F) Negative (G) Study success (H) Regulatory (I) Interim analysis (J) Ethical reason (K) Invalid reason (L) Study design (M) No context (N) Another study (O) Covid19

\centerline{\textit{- DC output -}}

(A) Insufficient enrollment (C) Business administrative

\subsubsection*{Relation extraction (RE)}
The RE task focuses on classifying the relation between any possible entity pairs within the same sentence. We adapt the relation labels from the original publications into descriptive language. We additionally include two adjacent sentences to provide more context information. Below is an example from the i2b2 2011 for coreference resolution on clinical named entities \cite{uzuner2012evaluating}:

\centerline{\textit{- RE Input -}}

According to the Medical text below, what is the co-reference relationship between the Person entity `Mr. Andersen' and the Person entity `who'? Choose from the following options.

Medical text: ... History of Present Illness: Mr. Andersen is a 71-year-old male with worsening anginal symptoms who underwent catheterization that showed severe three-vessel disease. He is presenting for revascularization . ...
Options: (A) `Mr. Andersen' refers to `who' (B) None of the above.

\centerline{\textit{- RE Output -}}

(A) `Mr. Andersen' refers to `who'

\subsubsection*{Multi-choice Question-answering (QA)}
The QA task aims to answer a research question regarding the medical text within a pre-defined answer set. The PubMedQA dataset consists of research questions about PubMed abstracts, with answers categorized as yes, no, or maybe \cite{jin2019pubmedqa}. The BioASQ includes biomedical questions with answers classified as yes or no \cite{tsatsaronis2015overview}. 

Directly applying our sequence classification prompt format for the QA task results in single-word multi-choice answers like \textit{yes} or \textit{no}. Instead, we transform the single-word options into descriptive sentences so that the QA output format is more straight-forward. We utilize one-shot learning with BioMistral to combine the question and each answer into a single statement. The one-shot example is randomly chosen from the PubMedQA train split, and the example output is written by human.

Below is an example of the QA input-output pair from the PubMedQA dataset, with descriptive multi-choice options. 

\centerline{\textit{- QA Input -}}

According to the medical literature below, Is there a connection between sublingual varices and hypertension? Choose from the following options. Only one option can be true.

Medical literature: BACKGROUND: Sublingual varices have earlier been related to ageing, smoking and cardiovascular disease. The aim of this study was to investigate whether sublingual varices are related to presence of ...

Options: (A) The answer is not mentioned in the text (\textit{maybe}). (B) There is a connection between sublingual varices and hypertension (\textit{yes}). (C) There is not a connection between sublingual varices and hypertension (\textit{no}).

\centerline{\textit{- QA Output -}}
(B) There is a connection between sublingual varices and hypertension (\textit{yes}).

\subsubsection*{Natural language inference (NLI)}
The NLI task utilizes a similar multi-choice prompt format to other sequence classification tasks. Below is an example from the BioNLI dataset \cite{bastan2022bionli}

\centerline{\textit{- NLI Input -}}

What is the relationship of the hypothesis with respect to the premise? Choose from the following options.

Premise: The administration of heparin with or without ACTH significantly decreased hepatic cholesterol content in catfish. In serum, heparin alone produced first hypercholesterolemia which was followed by hypocholesterolemia whereas it potentiated hypercholesterolemic action of ACTH three hours after administration.

Hypothesis: It is concluded that heparin inhibits the cholesterol-lowering action of ACTH in catfish.

Options: (A) neutral (B) entailment (C) contradiction

\centerline{\textit{- NLI Output -}}
(C) contradiction

\subsubsection*{Semantic text similarity (STS)}
We adapt the scoring criteria from the original publications and translate the numerical similarity scores into a descriptive sentences. Below is an example from the STS-B dataset \cite{wang2018glue}

\centerline{\textit{- STS Input -}}

How similar are the two sentences below? Choose from the following options.

Sentence 1: A plane is taking off.

Sentence 2: An air plane is taking off.

Options: (A) The two sentences are completely dissimilar. (B) The two sentences are not equivalent, but are on the same topic. (C) The two sentences are not equivalent, but share some details (D) The two sentences are roughly equivalent, but some important information differs / missing. (E) The two sentences are mostly equivalent, but some unimportant details differ. (F) The two sentences are completely or mostly equivalent, as they mean the same thing.

\centerline{\textit{- STS Output -}}
(F) The two sentences are completely or mostly equivalent, as they mean the same thing.

\subsubsection*{Natural language generation (NLG)}
We focus on the abstractive summarization task from NLG. Although abstractive summarization is different from our focus on NLU, it also requires in-depth document understanding, and thus we believe it can help improve NLU performance. We include three NLG datasets in the MNLU-Instruct: PubMedSum \cite{cohan-etal-2018-discourse}, CDSR \cite{guo2021automated}, and AciDemo \cite{yim2023aci}. PubMedSum has the input as the complete PubMed articles and the output as their abstracts. CDSR is a text simplification task that translates domain-specialized summaries into lay-user summaries. AciDemo is a task that summarizes doctor-patient dialogues into clinical note sections. Because the PubMedSum and AciDemo documents can be very lengthy, we only include instances with less than 800 words. Additionally, we restrict the output in PubMedSum to be at most half of its corresponding input word count to ensure that the PubMedSum splits contain high-quality summaries.

Below is an example from the AciDemo dataset.

\centerline{\textit{- NLG Input -}}

Summarize the relevant medical information from a dialogue between a doctor and a patient. The summary should be the objective exam section from the clinical note. Output None if no relevant information is found.

Dialogue:[doctor] hi alan , how are you ?

[patient] hi , good to see you .

[doctor] good to see you as well . are you ready to get started ?

[patient] ...

\centerline{\textit{- NLG Output -}}
PHYSICAL EXAMINATION 

Neck: Supple. 

No jugular venous distension.

Respiratory: Slight expiratory wheezing bilaterally.

Cardiovascular: Regular rate and rhythm. No murmurs.

Musculoskeletal: Trace edema in the bilateral lower extremities.

\subsection*{Baseline system with ICL for NER tasks} 
\label{sec:baseline_ICL}
Generalized LLMs do not automatically extract named entities in a unified format. To avoid confounding factors from different output formats and simplify NER evaluation, we utilize the same NER input-output format as described in Appendix \ref{sec:appdix_ner}. Additionally, we include a descriptive paragraph at the beginning of the input prompt to specify the output format: ``Your answer should use the following format, with one entity type per line. The span refers to the original text span from the Medical text. Output None if there is no such span. Use `...' to separate multiple spans.''

We also include two in-context examples to ensure the baseline system adheres to the desired output format. For each inference query, the 2-shot examples are randomly selected from the training split of each dataset. We ensure the outputs from the 2-shot examples are different from each other, to prevent bias towards a specific extraction response.
